# Supplementary material for: Bubble size statistics during reionization from 21-cm tomography
Source: arXiv:1706.00665 source file (2017-11-08)
Supplement: Supplementary file 1 [file appendix.tex]

\appendix

\section{Probability Distribution Function of sizes}
\label{app:PDF}

Let us consider the volume, $V$, as the metric for size of the ionized region and $N$ is the number of ionized regions of a particular size. If we randomly select a particular $V$, then the number of ionized regions of volume $V$ would lie between $N$ and $(N+{\mathrm d}N)$. The PDF of $V$ would be defined as,
\begin{equation}
\label{eq:PDF0}
P(V) dV = \frac{V(N+dN)-VN}{\int{VdN}}
=\frac{VdN}{\int{VdN}}
\end{equation}

The quantity in the denominator of the above equation is the scaling required for normalizing the PDF in order to give a physical meaning and can be comparable to different data. The bubble statistic methods(e.g. FOF) gives $V{\mathrm d}N/{\mathrm d}V$ as a function of $V$. The equation~\ref{eq:PDF0} can be rearranged as follows,
\begin{equation}
\label{eq:PDF1}
P(V) = \frac{V\frac{dN}{dV}}{\int{V\frac{dN}{dV}dV}} = V\frac{dn}{dV}
\end{equation}

In equation~\ref{eq:PDF1}, the scaling has been absorbed into a new quantity $n$. $P(V)$ represents the probability of finding an ionized region of size $V$ among the set of all ionized regions. The bigger ionized regions in the data cube are lesser in number. However, they contribute more to the global ionization. Therefore, we are interested in the fraction of the total ionized region that is constituted by bubbles in range ($V$,$V+\mathrm d V$). Thus, we can make a PDF of this quantity by normalizing the curve for each data cube.
\begin{equation}
\label{eq:PDF2}
p(V) = \frac{V^2\frac{dN}{dV}}{\int{V^2\frac{dN}{dV}dV}} = V^2\frac{dn}{dV}
\end{equation}

In the above equation, the quantity $n$ absorbs a different normalization factor. The other bubble statistic methods (e.g. MFP, SPA) have algorithm that determine the number of ionized region of a particular radius. In reality, the ionized regions in the data cube are volumes and they are not exactly spherical in shape. However, we can still use the radius as a proxy size metric to determine the fraction of ionized bubbles in the set of all ionized regions in the volume range ($\frac{4\pi}{3}R^3$, $\frac{4\pi}{3}(R+dR)^3$). These methods assume the ionized regions to be spherical in shape. The PDF determined from R has a similar definition as equation~\ref{eq:PDF0}.
\begin{equation}
\label{eq:PDF3}
\begin{aligned}
P(R) dR = \frac{R(N+dN)-RN}{\int{RdN}}
=\frac{RdN}{\int{RdN}}=Rdn \\
\Rightarrow P(R) = R \frac{dn}{dR}
\end{aligned}
\end{equation}

%%%%%%%%%%%%%%%%%%%%%%%%%%%%%%%%%%%%%%%%%%%%%%%%%%
